# Supplementary material for: Hypergraph Clustering for Finding Diverse and Experienced Groups
Source: arXiv:2006.05645 source file (2020-10-28)
Supplement: Supplementary file 1 [file supplement.tex]

% OPTIONAL TO INCLUDE (don't actually use anywhere)
\xhdr{Avoiding the non-regularized solution}
For $\beta$ values that are positive but very close to zero, the optimal solution to~\eqref{eq:ccilp} may still correspond to the optimal categorical edge clustering ($\beta = 0$) solution. In the interest of focusing on solutions that encourage a meaningful amount of diversity, we give a sufficient condition for guaranteeing when a node will deviate its $\beta = 0$ cluster assignment.

Let $x$ denote an arbitrary vector of variables satisfying constraints
in~\eqref{eq:ccilp}. The contribution of node $v$ to the fairness-regularization
term in our objective is $E(v, x) = \sum_{c \in L} d_v^c (1- x_v^c)$. Define
$X_0$ to be the set of optimal solutions to the categorical edge clustering
$\beta = 0$ objective. For $x^{ce} \in X_0$, the largest possible change in the
regularization term for a node $v$ among clusterings that are not $x^{ce}$ is
given by
\begin{equation}
\Delta E_v(x^{ce}) =\max_{x \notin X_0}E(v,x^{ce})-E(v,x).
\end{equation}
\begin{theorem} 
Let $x^{ce} \in X_0$. For an node $v \in V$ with total degree $d(v)$, if $\beta>\frac{d(v)}{\Delta E_v}$, the optimal solution to~\eqref{eq:ccilp} will place $v$ in different cluster that the one assigned to it by $x^{ce}$,
\end{theorem}
\begin{proof}
  The condition in the theorem implies that $\beta \Delta E_v>d(v)$, meaning that node $v$ will have an incentive to deviate from the cluster assignment given by $x^{ce}$, since the cost of staying in that assignment is greater than violating all of the hyperedges the node is in.
\end{proof}
